# Supplementary material for: Equilibrium Selection in Information Elicitation without Verification via Information Monotonicity
Source: arXiv:1603.07751 source file (2016-03-24)
Supplement: Supplementary file 1 [file additional_explanation.tex]

In this section, we will see for a specific family of mechanisms $\mathcal{F}$, for any $\mathcal{M}\in \mathcal{F}$, we can use our technique to modify $\mathcal{M}$ to a new mechanism $\mathcal{M}+$ that has truth-telling as \emph{weakly-quasi-focal}.

Falting\cite{radanovic2013robust} defines a \emph{decomposable} payment scheme (mechanism) as a payment scheme where each agent $i$'s total score his information score plus his prediction score and the information score does not depend on the agent's prediction report and the prediction score does not depend on the agent's information report (signal). Now we consider a family $\mathcal{F}$ of truthful mechanisms where (1) agents are asked to report his signal and prediction over other agents' reported signals; (2) the payment scheme is decomposable; (3) the prediction score for each agent $i$ is $PS(\hat{\sigma},\mathbf{p}_i)$ where $PS(\cdot,\cdot)$ is a strict proper scoring rule and $\mathbf{p}_i$ is agent $i$'s reported prediction. We will show if a truthful mechanism satisfies the above three conditions, then we can modify it to a mechanism that has truth-telling as \emph{weakly-quasi-focal}.

For any $DPS(PS(\cdot,\cdot))\in \mathcal{F}$, we use the same idea of designing our \emph{Disagreement Mechanism} to modify $DPS$: (a) divide agents into two non-empty groups to create a zero-sum game which has the same equilibria with $DPS$; (b) pay each agent $i$ an extra score that only depends on other agents. We will see this modified $DPS$ has truth-telling as \emph{weakly-quasi-focal} as well.

For each agent $i$, we define $payment_{DPS(PS(\cdot,\cdot))}(i,\mathbf{r})$ as the payment of agent $i$ given the report profiles of all agents is $\mathbf{r}$ under $DPS$ payment scheme. 

\paragraph{Modified DPS $\mathcal{DPS+}(PS(\cdot,\cdot))$}
\begin{enumerate}
\item Divide the agents into two non-empty groups-group A and group B. For group A, each agent $i_A$ receives a $$ score_{DPS}(i_A,\mathbf{r}) = payment_{DPS(PS(\cdot,\cdot))}(i_A,\mathbf{r})-\frac{1}{|A|}\sum_{j_B\in B} payment_{DPS(PS(\cdot,\cdot))}(j_B,\mathbf{r}) $$ For agents in group B, we use the same way to score them.  
\item Each agent $i$ is matched with two random agents $j,k$, the payment for agent $i$ is 
$$payment_{\mathcal{DPS+}(PS(\cdot,\cdot))}(i,\mathbf{r})=score_{DPS}(i,\mathbf{r})+score_C(r_j,r_k) $$
where $$score_C(r_j,r_k)=\left\{
\begin{aligned}
D^*(\mathbf{\hat{p}}_j,\mathbf{\hat{p}}_k) &  & \hat{\sigma}_j \neq \hat{\sigma}_k \\
-\sqrt{D^*(\mathbf{\hat{p}}_j,\mathbf{\hat{p}}_k)} &  & \hat{\sigma}_j = \hat{\sigma}_k 
\end{aligned}\right.
$$
\end{enumerate}

\begin{theorem}[Main Theorem]
Given any symmetric, non-zero, informative, fine-grained and ensemble prior, if the number of agents $n\geq 3$, $DPS+(PS(\cdot,\cdot))$ has truth-telling as a \emph{$(\tau_1,\tau_2,\gamma_1,\gamma_2)$-weakly-quasi-focal} equilibrium with $\tau_1(\gamma_1)=O(\sqrt[3]{\gamma_1})$, $\gamma_2(n)=O(\frac{m}{\sqrt{n}})$ and $\tau_2(n)=O(\sqrt[6]{\frac{m^2}{n})}$ (the constants we omit only depend on the first two moments of prior $Q$),
where $m$ is the number of signals, $n$ is the number of agents, and actually $\tau_1(\gamma_1)=\frac{1}{c_1}\sqrt[3]{\frac{\gamma_1}{c_2,c_3,c_4}}$, $\gamma_2(n)=\frac{4\sqrt{2}m}{\sqrt{n}}$ and $\tau_2^6(n)=\frac{128*m^2}{n c_1^6 (c_2 c_3 c_4)^2}$, $c_1 = \min_{s,t\in \Sigma} q(s|t)$, $c_2 = \min_{s,t\in \Sigma}Pr(s,t)$, $c_3 = \min_{u,v} \max_{s,t}||\frac{q(u|s)}{q(u|t)}-\frac{q(v|s)}{q(v|t)}||^2$, $c_4 = \min_{s,t,u} f''(\frac{q(u|s)}{q(u|t)})$ where $f(x)=(\sqrt{x}-1)^2$. 
 
\end{theorem}

\begin{proof}
Since $DPS$ is decomposable, for each agent $i$, his information score does not depend on his prediction which implies that his best response for prediction only needs to maximize his prediction score. Based on Claim~\ref{claim:best prediction} and the property of strict proper scoring rule, his best response for prediction would be $\theta_{-i} \mathbf{q}_{\sigma_i}$ (his belief for the likelihood of other agents' reported signals) given his private signal is $\sigma_i$. So at any equilibrium $s$ under $DPS$, we have $s=s_{BP}$ which implies $\textit{ClassificationScore}(s)= \textit{TotalDivergence}(s_{BP})$ in $DPS$. So our main lemma still holds, then the rest of the proof follows from our previous proof for our main theorem.

\end{proof}

The multi-RBTS mechanism in \cite{radanovic2013robust} is in $\mathcal{F}$, the modified multi-RBTS mechanism has truth-telling as \emph{weakly-quasi-focal} while this mechanism requires additional assumption (self-predicting assumption\cite{radanovic2013robust}: any agent $i$ will believe another agent $k$ is most likely to observe a certain value x when she herself also observes this value) for prior to make truth-telling an equilibrium and our \emph{Disagreement Mechanism} does not need this additional assumption.
